# Supplementary material for: The impact of spurious imaginary phonon modes on thermal properties of Metal-organic Frameworks
Source: arXiv:2602.07295 source file (2026-05-28)
Supplement: Supplementary file 1 [file Supplementary_Information.pdf]

# Supporting Information: The impact of spurious imaginary phonon modes on thermal properties of Metal-organic Frameworks

Prathami Divakar Kamath[1,2], Kristin A. Persson[1,2,†]

[1]Department of Materials Science & Engineering, University of California, Berkeley, CA, USA

[2]Materials Sciences Division, Lawrence Berkeley National Laboratory, Berkeley, CA, USA

† Corresponding author *

E-mail: kapersson@lbl.gov

## 1 Mode Contribution of low frequency phonons

As discussed in the main text, here we provide proof for why a full contribution can be assumed for phonons in the 0-3 THz range corresponding to the typical region of acoustic modes and low frequency optical modes at 300K and higher temperatures. The per mode contribution to the total heat capacity has been shown for 3 unique low-frequencies 1, 2 and 3 THz respectively in the Figure. For frequency $\nu$ =1 and 2 THz, the $\frac{C_v}{k_B}$ saturates to 1 at temperatures below room temperature. As seen from the band diagrams the acoustic

modes and low frequency optical modes which are often found to be the spurious imaginary modes have physical frequencies within this range. At moderate frequencies like 3THz, the temperature for saturation shifts to $\sim$ 300 or above, but this frequency is generally above the range of acoustic modes for MOFs. Therefore, the approximation of full $k_B$ contribution for the imaginary modes corresponding to frequencies in this range proposed in this work holds.

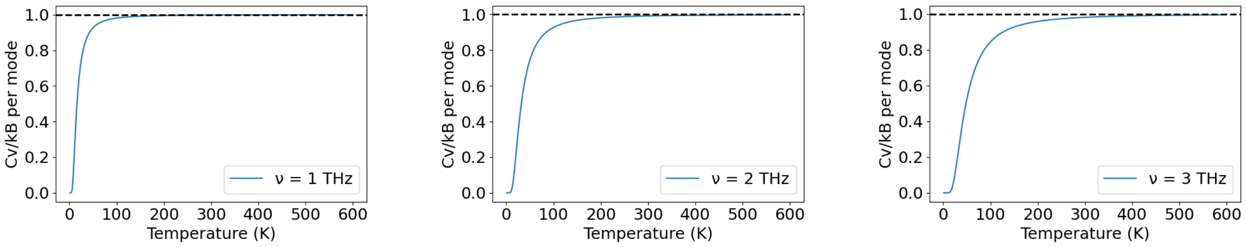


(a) (b) (c)

Figure S1: Supplementary Figure S1. This figure shows for low-frequency ($\nu$) modes (a) 1 THz (b) 2 THz and (c) 3 THz modes can be approximated to be fully active at 300K and higher temperatures as $C_v \sim k_B$.

# 2 Structural Details of the Chosen MOFs

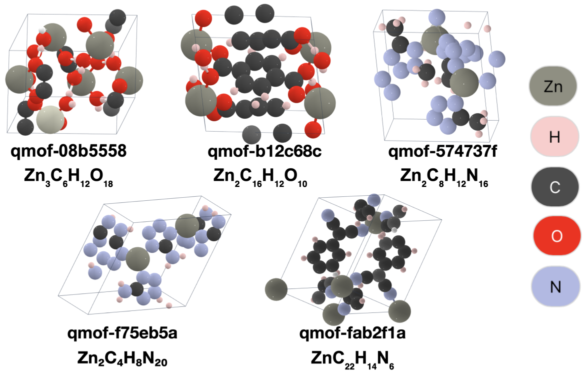


Figure S2: Supplementary Figure S2. The structures of the five chosen MOFs from the forty MOFs sampled by Yue *et al.*[S1] from QMOF[S2,S3]

# 3 Phonon Band diagrams from MACE-MP-MOF0 with 0% imaginary modes

The Figure S3 demonstrates the nature of the 0-3 THz frequency phonon modes comprising of acoustic modes ($\sim<$ 2 THz) and some low frequency optical modes $<$ 3 THz predicted by MACE-MP-MOF0.[S4]

# 4 Benchmarking of MLIPs with DFT data containing spurious imaginary modes

In addition to the two MOFs discussed in the main text, here are the results of the remaining three MOFs which shows the generalization of the proposed solution to all systems and the artificially better performance of the Yue *et al.*[S1] **MLP** due to the presence of imaginary modes in the MLP as well as the reference Data. Figure S4 (c) shows a unique example of the MOF "qmof-f75eb5a" where the Yue *et al.*[S1] **MLP** overestimates the $C_v$ data even relative to the corrected contribution DFT data implying that the intrinsic overestimation from the model is larger and that the % imaginary modes from the **MLP** are artificially reflecting smaller overestimation from DFT data. This implies that even if DFT data were free of spurious imaginary modes its important to check for the imaginary modes from the MLIPs too to confirm that the low errors are intrinsic to the model and not due to imaginary modes.

# 5 Propagation of errors from $C_v$

$C_v$ is the most experimentally relevant property and hence, was the focus of the main text. For theoretical insights on the effect of other derived thermodynamic properties under the canonical ensemble, the errors in F (Helmoltz Free Energy), S (Entropy), and U (Harmonic

Phonon Energy) due to 1.03% spurious imaginary modes relative to 0% from DFT in MOF-74 are shown in Figure S5.

$$F(T) = \sum_{\mathbf{q},\nu} \left[ \frac{1}{2}\hbar\omega_{\mathbf{q}\nu} + k_B T \ln\left(1 - e^{-\hbar\omega_{\mathbf{q}\nu}/k_B T}\right) \right] \tag{1}$$

$$U(T) = \sum_{\mathbf{q},\nu} \left[ \frac{1}{2}\hbar\omega_{\mathbf{q}\nu} + \frac{\hbar\omega_{\mathbf{q}\nu}}{e^{\hbar\omega_{\mathbf{q}\nu}/k_B T} - 1} \right] \tag{2}$$

$$S(T) = k_B \sum_{\mathbf{q},\nu} \left[ \frac{\hbar\omega_{\mathbf{q}\nu}/k_B T}{e^{\hbar\omega_{\mathbf{q}\nu}/k_B T} - 1} - \ln\left(1 - e^{-\hbar\omega_{\mathbf{q}\nu}/k_B T}\right) \right] \tag{3}$$

All of these quantities can be expressed in terms of $C_v$ as per equations 7, 6 and 4. As shown in Figure S5 (a) the underestimation in U continuously increases with temperature (T) because the errors from $C_v$ keep accumulating with T as per equation 4. On the other hand, the errors in S are much larger at lower temperatures because of a $T^2$ dependence of $\frac{C_v}{T}$. As the % underestimations in S are much larger than U at higher temperatures due to the -TS(T) contribution the % errors in F turn into overestimation.

$$U(T) = U_0 + \int_0^T C_V(T')\, dT' \tag{4}$$

where

$$U_0 = \frac{1}{2} \sum_{\mathbf{q},j} \hbar\omega_{\mathbf{q}j} \quad \text{(zero-point energy).} \tag{5}$$

$$S(T) = \int_0^T \frac{C_V(T')}{T'}\, dT' \tag{6}$$

$$F(T) = U(T) - TS(T) \tag{7}$$

## References


(S1) Yue, Y.; Mohamed, S. A.; Loh, N. D.; Jiang, J. Toward a Generalizable Machine-Learned Potential for Metal–Organic Frameworks. *ACS Nano* **2025**, *19*, 933–949.

(S2) S., R. A.; M., I. S.; D., R.; Z., Y.; A., A.-G.; L., G.; M., N. J.; Q., S. R. Machine learning the quantum-chemical properties of metal–organic frameworks for accelerated materials discovery. *Matter* **2021**, *4*, 1578–1597.

(S3) S., R. A.; V., F.; P., H.; T., O. C.; K., H. M.; G., T. D.; A., P. K.; M., N. J.; Q., S. R. High-throughput predictions of metal–organic framework electronic properties: theoretical challenges, graph neural networks, and data exploration. *npj Comput. Mater.* **2022**, *8*, 112.

(S4) M., E. A.; D., K. P.; T., J. I.; S., R. A.; F., Z.; A., P. K. Machine learned potential for high-throughput phonon calculations of metal–organic frameworks. *npj Comput. Mater.* **2025**, *11*, 125.

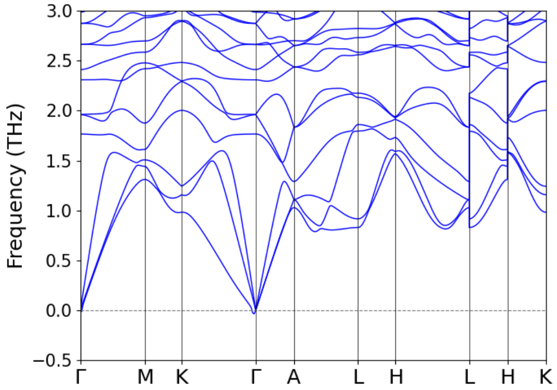


**(a)**

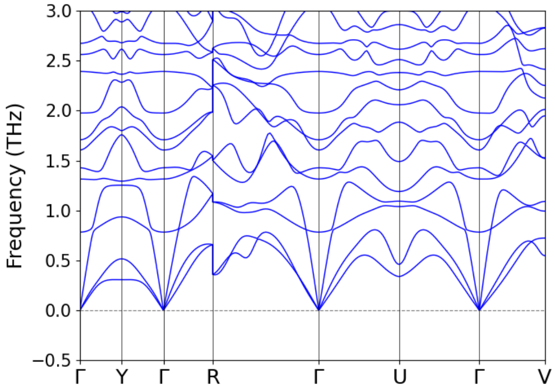


**(b)**

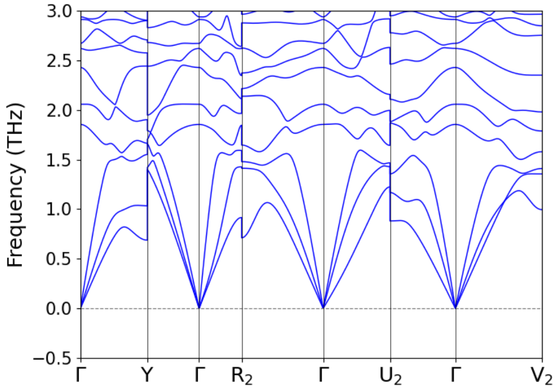


**(c)**

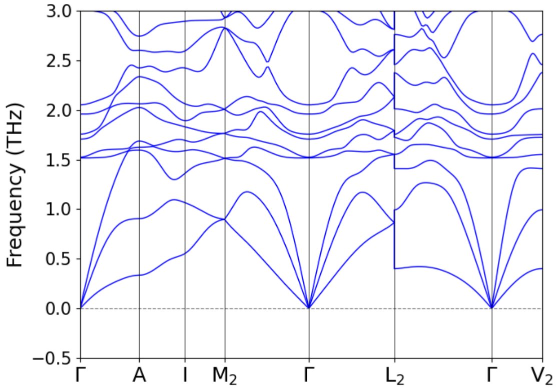


**(d)**

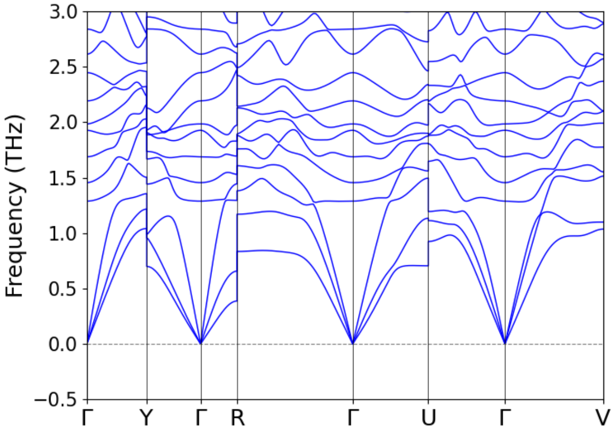


**(a)**

Figure S3: Supplementary Figure S3. This figure shows for low-frequency ($<$ 3 THz) phonon band diagrams for the five chose MOFs from QMOF[S2,S3] (a) "qmof-08b5558" (b) "qmof-574737f" (c) "qmof-b12c68c" (d) "qmof-f75eb5a" and (e) "qmof-fab2f1a". MACE-MP-MOF0 produces imaginary-mode-free data for all these MOFs without needing elimination procedures.

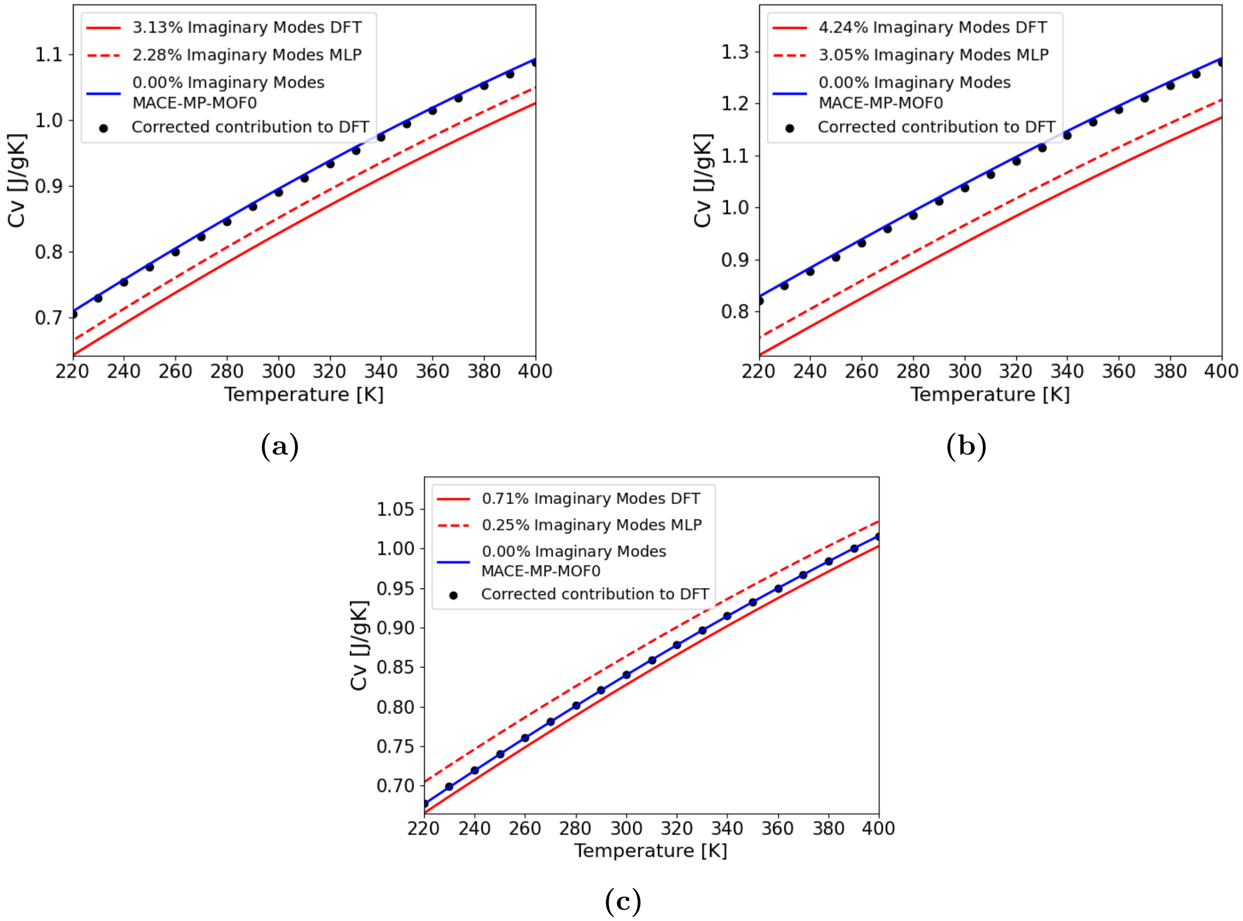


Figure S4: Supplementary Figure S4. This figure shows the misrepresentation of property-based accuracy from **MLP** when the underlying spurious imaginary modes are not accounted for benchmarking MLIPs with DFT with the examples of (a) "qmof-b12c68c" (b) "qmof-fab2f1a" and (c) "qmof-f75eb5a"

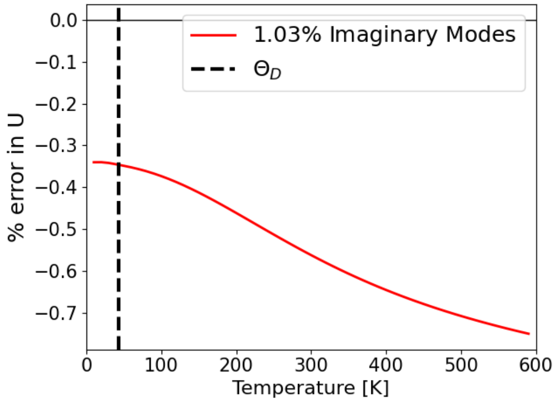


**(a)**

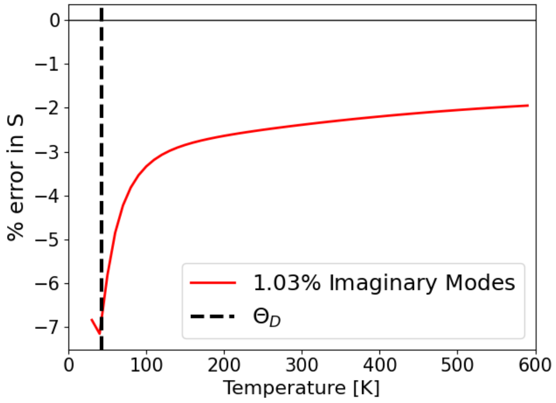


**(b)**

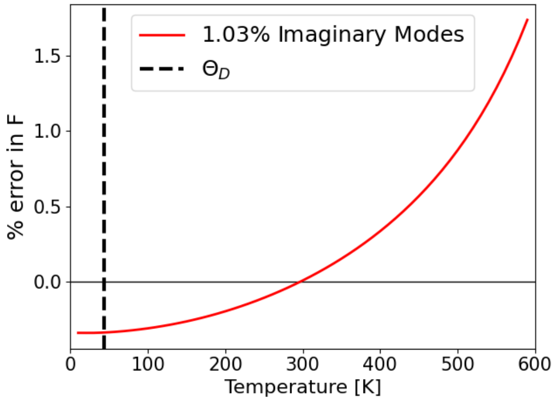


**(c)**

Figure S5: Supplementary Figure S5. This figure shows the percentage deviations in (a) U, (b) S and (c) F for MOF-74 for $C_v$ errors discussed in the Figure 1 of the main text.
